# Supplementary material for: Single copy of the Ricci flow
Source: arXiv:2202.09874 source file (2022-02-20)
Supplement: Supplementary file 1 [file appendix1.tex]

\section{Appendix} \label{sec:appendix}
